# Supplementary material for: AI on the Edge: Rethinking AI-based IoT Applications Using Specialized Edge Architectures
Source: arXiv:2003.12488 source file (2020-03-27)
Supplement: Supplementary file 1 [file appendix.tex]

\begin{figure}
    \centering
    \includegraphics[width=0.4\textwidth]{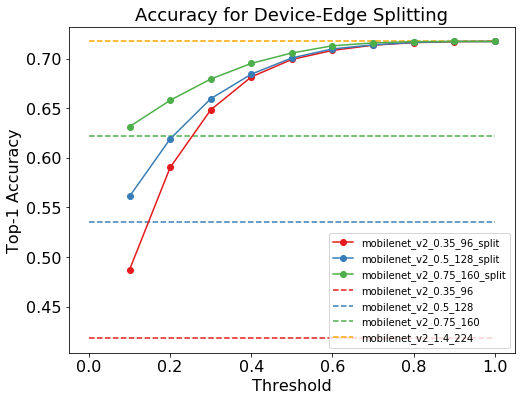}
    \caption{Accuracy vs. threshold for hierarchically distributed computing architecture with a small model on device and large model on edge with a NCS2 accelerator. On device, we use MobileNet V2 with depth multiplier 0.35 and input size 96; On edge, we use the same model with depth multiplier 1.4 and input size 224. The horizontal dashed lines are the accuracy of these models respectively. Accuracy is computed using ImageNet\cite{imagenet_cvpr09} validation set.
}
    \label{fig:acc_device_edge}
\end{figure}

\begin{figure}
    \centering
    \includegraphics[width=0.4\textwidth]{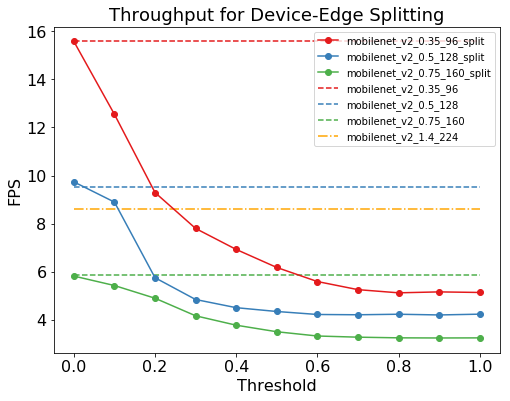}
    \caption{Throughput vs. threshold for hierarchically distributed computing architecture. The setup is the same as figure \ref{fig:acc_device_edge}}
    \label{fig:throughput_device_edge}
\end{figure}

\begin{figure}
    \centering
    \includegraphics[width=0.4\textwidth]{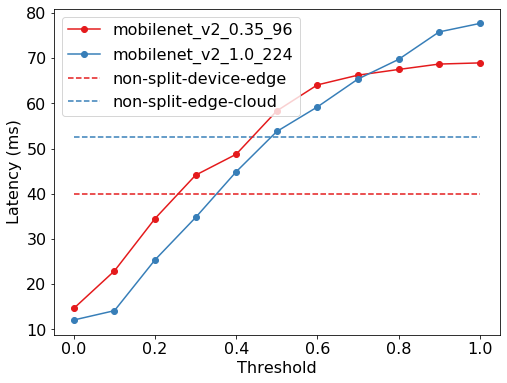}
    \caption{Latency vs. threshold for hierarchically distributed computing architecture. The setup is the same as figure \ref{fig:acc_device_edge}}
    \label{fig:latency_device_edge}
\end{figure}

\begin{figure}
    \centering
    \includegraphics[width=0.4\textwidth]{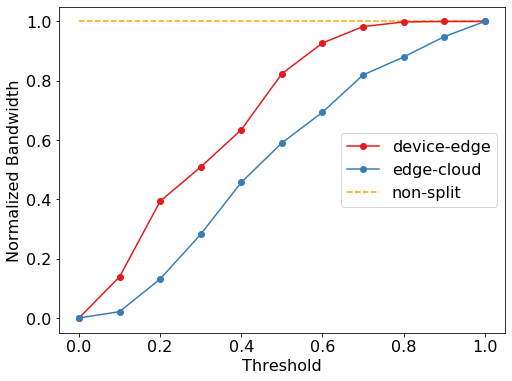}
    \caption{Bandwidth vs. threshold for hierarchically distributed computing architecture. The setup is the same as figure \ref{fig:acc_device_edge}}
    \label{fig:bandwidth_device_edge}
\end{figure}

\begin{figure}
    \centering
    \includegraphics[width=0.4\textwidth]{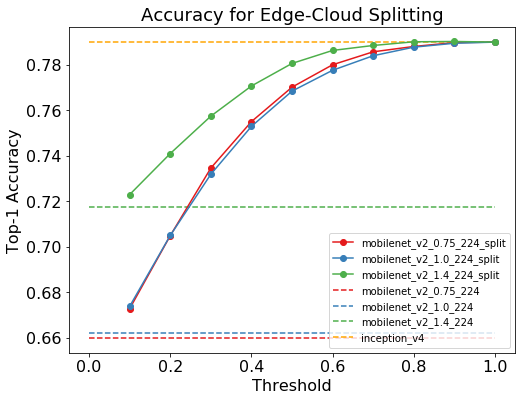}
    \caption{Accuracy vs. threshold for hierarchical distributed computing architecture where the small-footprint models are located on edge devices and the more sophisticated model is located on the cloud}
    \label{fig:acc_edge_cloud}
\end{figure}

\begin{figure}
    \centering
    \includegraphics[width=0.4\textwidth]{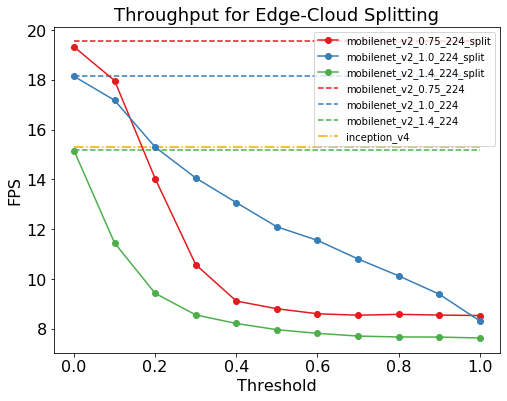}
    \caption{Throughput vs. threshold for hierarchical distributed computing architecture with same setup as \ref{fig:acc_edge_cloud}}
    \label{fig:throughput_edge_cloud}
\end{figure}

\begin{figure}
    \centering
    \includegraphics[width=0.4\textwidth]{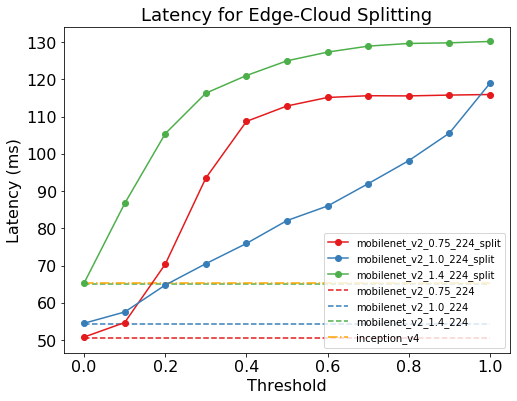}
    \caption{Latency vs. threshold for hierarchical distributed computing architecture with same setup as \ref{fig:acc_edge_cloud}}
    \label{fig:latency_edge_cloud}
\end{figure}

\begin{figure}
    \centering
    \includegraphics[width=0.4\textwidth]{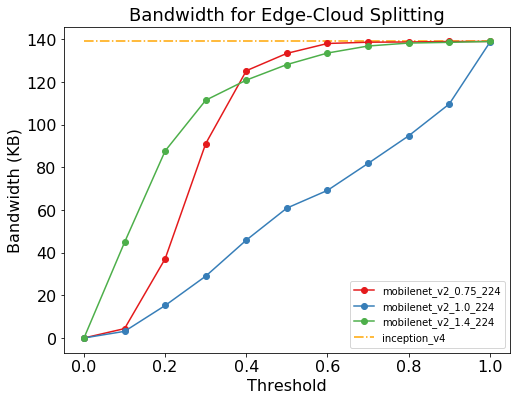}
    \caption{Bandwidth vs. threshold for hierarchical distributed computing architecture with same setup as \ref{fig:acc_edge_cloud}}
    \label{fig:bandwidth_edge_cloud}
\end{figure}

\begin{figure}
    \centering
    \includegraphics[width=0.4\textwidth]{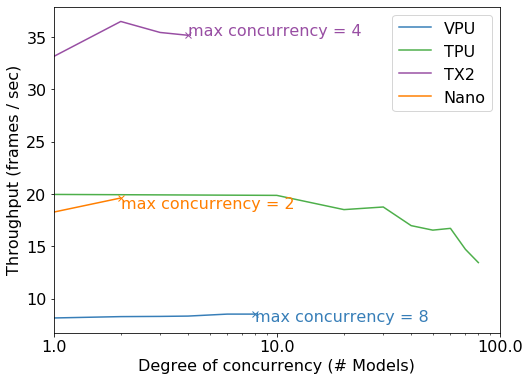}
    \caption{Throughput in frames per second vs. size of models loaded to device. NCS2 throws out of memory error when requested memory size excced its limit. EdgeTPU allows user requesting memory size exceed its limit and do context switch at runtime, which hurts its performance. }
    \label{fig:throughput_vs_size}
\end{figure}
